# Supplementary material for: Provable Regret Bounds for Deep Online Learning and Control
Source: arXiv:2110.07807 source file (2022-02-16)
Supplement: Supplementary file 1 [file weak_realizability.tex]

\section{Weak Realizability}
\begin{definition}
A function class $\H$ is $(k, \eps)$ -realizable (for scalar functions) if for any $\{(x_i, y_i)\}_{i=1}^k$ where $x_i\in \mathbb{S}, y_i\in [-1, 1]$ there exists a function $f\in \H$ such that $$
\sum_{i=1}^k (y_i - f(x_i))_2^2 \le \eps.
$$
\end{definition}

Let $\H$ be the class of deep neural networks as specified in Section \ref{sec:dnn_def}, with parameters $\theta \in B(R)$, then we have the following lemma,
\begin{lemma}
For $R = O\left(\frac{k^3}{\sqrt{m}}\right)$, $\H$ is $(k, \eps)$ weakly realizable.
\end{lemma}

\paragraph{Approach 1:} According to Yuanzhi's paper, near initialization, the gradient of loss with respect to the parameters is lower bounded by the function value of the loss. Coupled with the fact that the loss function is semi-smooth with respect to neural network parameters, one can show that gradient descent always makes progress. Therefore, one can fit any label near initialization to arbitrary accuracy. Finally, it is shown that the parameters move at most $O(1/\sqrt{m})$. 

\paragraph{Approach 2:} Constructive proof: for given input $x \in \mathbb{S}$ and target output $y \in [-1, 1]$, construct $\theta$ such that $f(x; \theta) = y$ and $\theta \in B(R)$. Need to show this is possible for some $R = O(1/\sqrt{m})$.

For the deep network model as in \eqref{eq:deep_nn} (the scalar case), a suggestions for such a construction. Let $\theta_1$ denote the initial parameter, and $f(x; \theta_1) = y_1$. The idea is to reach target $y$ from $y_1$ using only the last layer, i.e. take $\theta^h = \theta_1^h$ for $1\leq h < H$. This means that the output at $H-1$ layer is identical, $x^{H-1} \equiv x^{H-1}_1$, and we need to choose $\theta^H$ such that
\begin{align*}
    f(x; \theta) - f(x; \theta_1) = a^{\top} (x^H - x_1^H) = y - y_1 ~.
\end{align*}
Take $i \in \argmax_{j \in [m]} \{ a_j \cdot \text{sgn}(y-y_1) : x^H_1[j] > 0\}$, and modify the output via only index $i$: $\theta^H[j] \equiv \theta^H_1[j]$ for $j \neq i$. This leads to
\begin{align*}
    x^H[i] - x^H_1[i] = (\theta^H[i] - \theta_1^H[i])^{\top} x^{H-1} = (y-y_1) / a_i > 0 ~.
\end{align*}
Finally, this means the target parameter to choose is $\theta^H[i]=  \theta^H_1[i] + C \cdot x^{H-1}$ where $C > 0$ is a constant given by $C = \frac{y-y_1}{a_i \|x^{H-1}\|^2}$. Furthermore, we know that $\theta \in B(R)$ means $R \geq C \cdot \| x^{H-1} \|$. Note that $\|y-y_1\|$ is on the order of $\sqrt{m}$, $\|x^{H-1}\|$ is a constant, then $R$ should be on the order of $\sqrt{m}$ -- $m$ times larger than the desired scale. What is wrong with the construction?

Well, the same logic for the $2$-layer case gets us to $R$ being on the scale of $\sqrt{m}$ (instead of desired constant scale), as the corresponding expression becomes $y = \frac{1}{\sqrt{m}} (\theta[r] - \theta_1[r])^{\top} x$.

\begin{enumerate}
    \item Depth: the construction ignores the first $H-1$ layers of the parameters, they are not leveraged in changing the output value. This shouldn't be true since the statement should hold for the $2$-layer case too where $H=1$.
    \item Scaling: Putting the $\frac{1}{\sqrt{m}}$ scaling factor in front of the output in the discussed case simply makes $y-y_1$ to a constant scale but adds an extra $\sqrt{m}$ in the expression for $C$, no difference again.
    \item Symmetric initialization: this would make $y_1=0$ instead of around $\sqrt{m}$, and end up shaving off a $\sqrt{m}$ factor for $R$.
\end{enumerate}

There is still an extra $\sqrt{m}$ factor as in the $2$-layer case. This factor is extra given the explanation in approach 1. Need to find what's off about this construction (except that we need symmetric initialization in the deep case).
